# Supplementary material for: Robust Graph Neural Networks via Unbiased Aggregation
Source: arXiv:2311.14934 source file (2024-11-09)
Supplement: Supplementary file 1 [file convergence.tex]

% NOTE: overlapped with IRLS
\section{tmp: Conervgence}
    \subsection{Upperbound}
    Now we prove the theorem
    \subsection{Preconditioning and convergence}
        The upper bound of \autoref{eq:energy_rw_appnp} has been found to be \autoref{eq:converge_mm_obj}
        % \begin{equation}\label{eq:converge_mm_obj}
        %     \sumedge \mW_{ij}  \|\frac{\vf_i}{\sqrt{d_i}} - \frac{\vf_j}{\sqrt{d_j}}\|_2^2  + \hat{\lambda}\sumnode \|\vf_i - \vf_i^{(0)}\|_2^2, 
        % \end{equation}
        which is a convex function of $\vf$. Its gradient is
        \begin{equation}
            2 (\text{diag}(\vq) - \mW\odot\tilde{\mA}) \mF^{(k)} + 2 \hat{\lambda} \mF^{(k)} - 2 \hat{\lambda} \mF^{(0)}
        \end{equation}
        as was given before.

        \paragraph{Convergence}
            Now we prove that the convergence with the step size in \autoref{eq:rw_update_f2} is guaranteed by proving the bounded spectrum of $\hat{\mQ}^{-\frac{1}{2}}(\mW\odot\tilde{\mA})\hat{\mQ}^{-\frac{1}{2}}$ since it is symmetric positive semi-definite.
            % This seems promising since the spectrum of the normalized degree matrix is bounded by 1
            
            % As we know, the symmetrically normalized adjacent matrix $\tilde{A}$ is bounded by $1$. Denote the eigenvector with the largest eigenvalue of $\hat{\mQ}^{-1}(\mW\odot\tilde{\mA})$ as $\vy$, 
            % \begin{align}
            %     (\hat{\mQ}^{-1}(\mW\odot\tilde{\mA})\vy)_j
            %     &=
            %     \sum_{i} \hat{\mQ}^{-1}_{jj}(\mW\odot\tilde{\mA})_{ji} \vy_i
            %     =
            %     \mu \vy_j \\
            %     &=
            %     \frac{d_j}{\sum_k \mW_{jk} \mA_{jk} + \hat{\lambda}} \sum_{i} \mW_{ji} \tilde{\mA}_{ji} \vy_i \\
            %     &\le
            %     \frac{d_j}{\sum_k \mW_{jk} \mA_{jk}} \sum_{i} \mW_{ji} \tilde{\mA}_{ji} \vy_i \label{eq:converge_failure1}
            % \end{align}
            % Ah, I'm stuck here.
            % \par
            % If $\Tilde{\mA}$ were random walk normalized, i.e. $\tilde{\mA'}_{ij} = \frac{\mA_{ij}}{\sum_k \mA_{ik}} = \frac{\mA_{ij}}{d_i}$ , then following from \autoref{eq:converge_failure1},
            % \begin{equation}
            %     \mu\vy_j \le \frac{\sum_k \mW_{jk}\mA_{jk}\vy_k}{\sum_k \mW_{jk}\mA_{jk}} \le \max_k \vy_k
            % \end{equation}
            % for any component $j$. Choose the largest component $j = \text{argmin}_k \vy_k$ and we immediately get $\mu \le 1$. 
            % \par
            
            Notice that $\bar{L}=\text{diag}(\vq) - (\mW\odot \tilde{\mA})$ is positive semi-definite \footnote{This can be seen by writing down the upper bound of the objective $\mathcal{L^*} = \tr(\mF^{\top} (\text{diag}(\vq) - \mW\odot\tilde{\mA}) \mF) + \|\mF - \mF^{(0)}\|_{\mathcal{F}}^2$ and noticing the first term $ \tr(\mF^{\top} \bar{L} \mF)$ expands to $\sumedge \mW_{ij}\|\frac{\vf_i}{\sqrt{d_i}} + \frac{\vf_j}{\sqrt{d_j}}\|_2^2 \ge 0$.}, so $\forall\vx, \vx^\top (\text{diag}(\vq) - (\mW\odot\tilde{\mA}))\vx \ge 0$ and thus 
            \begin{equation}
                \forall\vx, 1 \ge \frac{\vx^\top (\mW\odot\tilde{\mA}) \vx}{\vx^\top\text{diag}(\vq)\vx}.
            \end{equation}
            Extract a $\hat{\mQ}^{\frac{1}{2}} = \text{diag}(\vq)^{\frac{1}{2}}$ from $(\mW\odot\Tilde{\mA})$ in the previous inequality, 
            % \begin{equation}
            %     1 \ge \frac{\vy^\top \text{diag}(\vq)^{\frac{1}{2}} \left(\text{diag}(\vq)^{-1}(\mW\odot\tilde{\mA})\right)\text{diag}(\vq)^{-\frac{1}{2}} \vy}{\vy^\top \vy} = \frac{\sum_i \lambda_i x_i^2}{\sum_i w_i x_i^2}.
            % \end{equation}
            \begin{equation}
                \forall\vx, 1 \ge \frac{\vx^\top \hat{\mQ}^{\frac{1}{2}} \left(\hat{\mQ}^{-\frac{1}{2}} (\mW\odot\tilde{\mA}) \hat{\mQ}^{-\frac{1}{2}} \right) \hat{\mQ}^{\frac{1}{2}} \vx}{\vx^\top\hat{\mQ}^{\frac{1}{2}}\hat{\mQ}^{-\frac{1}{2}} \text{diag}(\vq) \hat{\mQ}^{-\frac{1}{2}}\hat{\mQ}^{\frac{1}{2}} \vx}.
            \end{equation}
            Pick $\xi = \hat{\mQ}^{\frac{1}{2}}\vx$ to be the eigenvector corresponding to the largest eigenvalue of $\text{diag}(\vq + \hat{\lambda})^{-\frac{1}{2}} (\mW\odot\tilde{\mA}) \text{diag}(\vq + \hat{\lambda})^{-\frac{1}{2}}$, so that
            \begin{equation}\label{eq:convergence_bounded_spectrum_of_WA}
                1 \ge \frac{\lambda_{\text{max}} \xi^\top \xi}{\xi^\top \text{diag}(\frac{\vq}{\vq + \hat{\lambda}}) \xi} \ge \lambda_\text{max},
            \end{equation}
            as long as $\lambda_{\text{max}}\ge 0$, otherwise $\lambda_{\text{max}} \le 0$. In either case we have $\lambda_{\text{max}} \le 1$.
            \par
            Similarly, since $\vf_i^\top(\text{diag}(\vq) + (\mW\odot \tilde{\mA}))\vf_j = \sumedge \mW_{ij}\|\frac{\vf_i}{\sqrt{d_i}} + \frac{\vf_j}{\sqrt{d_j}}\|_2^2 \ge 0$, 
            \begin{equation}\label{eq:convergence_WA_spectrum_bound-1}
                \forall\vx, -1 \le \frac{\vx^\top (\mW\odot\tilde{\mA}) \vx}{\vx^\top\text{diag}(\vq)\vx},
            \end{equation}
            and thus $\lambda_{\text{min}} \ge -1$.
            Therefore, combining the previous result, we proved that
            \begin{equation}
                -1 \le \lambda \le 1.
            \end{equation}
            % , so $\lambda_{\text{min}}\ge 0$, and hence convergence. However, the convergence criteria here only works if the minimization of \autoref{eq:converge_mm_obj} is carried out until convergence, but it does not tell us what happens if the minimization step like \autoref{eq:converge_mm_update_Richardson} is carried out only once. 

        \subsection{Guaranteed Descent}
            In order for the majorization-minimization method to work robustly, one may require in each majorize-minimize step the objective \autoref{eq:energy_rw_appnp} decreases. Note that the majorization upper bound \autoref{eq:converge_mm_obj} coincides with \autoref{eq:energy_rw_appnp} when $\mW_{ij} = \frac{\partial \rho(z_{ij}^2)}{\partial z_{ij}^2}$, and therefore in the $k$-th majorization, after excluding irrelevant constants,
            \begin{align}
                & \hat{\energy} = \sumedge \mW_{ij}  \|\frac{\vf_i}{\sqrt{d_i}} - \frac{\vf_j}{\sqrt{d_j}}\|_2^2  + \hat{\lambda}\sumnode \|\vf_i - \vf_i^{(0)}\|_2^2\\ 
                \ge & \energy  =  \sumedge \rho\left(\|\frac{\vf_i}{\sqrt{d_i}} - \frac{\vf_j}{\sqrt{d_j}}\|_2\right) + \hat{\lambda} \sumnode \|\vf_i - \vf_i^{(0)}\|_2^2
            \end{align}
            where the equality holds when $\vf = \vf^{(k)}$. Hence, we only need to prove that $\hat{\energy}^{(k+1)} \le \hat{\energy}^{(k)}$ to show $\energy^{(k+1)} \le \hat{\energy}^{(k)}_{\star} \le \hat{\energy}^{(k)} = \energy^{(k)}$
            where $\hat{\energy}^{(k)}_{\star}$ means the upper bound of the objective after the minimization procedure, which can consist of one or multiple steps.
            \par
            Now we prove that the normalization of $\mW \odot \mA$ and stepsize $\eta = \frac{1}{2}$ used in \autoref{eq:rw_update_f2} is sufficient for $\hat{\energy}^{(k)}_{\star} = \hat{\energy}^{(k)}(\mF^{(k)} - \frac{1}{2}\hat{\mQ}^{-1}\nabla\energy(\mF^{(k)})) \le \hat{\energy}^{(k)}(\mF^{(k)})$. We start by noticing the $\beta$-continuity of $\Hhat$. To get a tighter upper bound, we deviate from the ordinary approach. First, we have 
            \begin{align}
                &\| \hat{\mQ}^{-\frac{1}{2}} \left(\nabla\Hhat(\vx) - \nabla\Hhat(\vy)\right)\| \\
                =& 2\|  \hat{\mQ}^{-\frac{1}{2}} \left( \text{diag}(\vq) + \hat{\lambda} \mI - \mW\odot\tilde{\mA}\right) \hat{\mQ}^{-\frac{1}{2}} \hat{\mQ}^{\frac{1}{2}}(\vx - \vy)\| \\
                =& 2\| \hat{\mQ}^{-\frac{1}{2}} \left(\text{diag}(\vq) + \hat{\lambda} \mI - \mW\odot\tilde{\mA}\right) \hat{\mQ}^{-\frac{1}{2}} \hat{\mQ}^{\frac{1}{2}}(\vx - \vy)\|\\
                \label{subeq:convergence_singularvalue}\le & 2 \| \hat{\mQ}^{\frac{1}{2}}(\vx - \vy)\| \| \hat{\mQ}^{-\frac{1}{2}} \left(\text{diag}(\vq) + \hat{\lambda} \mI - \mW\odot\tilde{\mA}\right) \hat{\mQ}^{-\frac{1}{2}}\|\\ 
                \label{subeq:convergence_sinval_lessthan1}\le & 4\| \hat{\mQ}^{\frac{1}{2}} (\vx - \vy) \|,
            \end{align}
            where \autoref{subeq:convergence_singularvalue} follows from the definition of $l_2$ norm, and \autoref{subeq:convergence_sinval_lessthan1} follows directly from the conclusion in \autoref{eq:convergence_bounded_spectrum_of_WA} that any eigenvalue of $\hat{\mQ}^{-\frac{1}{2}}(\mW\odot\tilde{\mA})\hat{\mQ}^{-\frac{1}{2}}$ falls into $[-1, 1]$, so any eigenvalue of $\mI - \hat{\mQ}^{-\frac{1}{2}}(\mW\odot\tilde{\mA})\hat{\mQ}^{-\frac{1}{2}}$ falls into $0, 2$ and so does that of $\hat{\mQ}^{-\frac{1}{2}}(\hat{\mQ} - \mW\odot\tilde{\mA})\hat{\mQ}^{-\frac{1}{2}}$. These matrices are all symmetric and thus the eigenvalues correspond to their singular values.
            Then using Cauchy-Schwartz inequality and the inequality above,
            \begin{align}\label{eq:convergence_beta_sm_bound_1}
               &  |\Hhat(\vx) - \Hhat(\vy) - \nabla \Hhat(\vy)^\top (\vx - \vy)|  \\
               = &| \int_0^1 (\nabla \Hhat(\vy + t(\vx - \vy))^\top - \nabla \Hhat(\vy)^\top) (\vx - \vy) dt | \\
               = & |\int_0^1 (\hat{\mQ}^{-\frac{1}{2}}(\nabla \Hhat(\vy + t(\vx - \vy)) - \nabla \Hhat(\vy)))^\top \hat{\mQ}^{\frac{1}{2}} (\vx - \vy) dt|  \\
               \le &| \int_0^1 \| \hat{\mQ}^{-\frac{1}{2}}(\nabla \Hhat(\vy + t(\vx - \vy)) - \nabla \Hhat(\vy)) \| \| \hat{\mQ}^{\frac{1}{2}} (\vx - \vy) \| dt|  \\
               \le & \int_0^1 4t \|\hat{\mQ}^{\frac{1}{2}} (\vx - \vy) \| \| \hat{\mQ}^{\frac{1}{2}} (\vx - \vy) \| dt \\
               = & 2\|\hat{\mQ}^{\frac{1}{2}} (\vx - \vy) \| \| \hat{\mQ}^{\frac{1}{2}} (\vx - \vy) \|.
            \end{align}
            Note that 
            \begin{equation}
                \Hhat(\vx) - \Hhat(\vy) - \nabla \Hhat(\vy)^\top (\vx - \vy) \le |\Hhat(\vx) - \Hhat(\vy) - \nabla \Hhat(\vy)^\top (\vx - \vy)|, 
            \end{equation}
            and by taking $\vx = \vy - \eta \hat{\mQ}^{-1}\nabla \Hhat(\vy)$, 
            % In fact x - y can be any vector, we constrain it on this direction because we know that this is the optimal set. The \eta - \eta^2 we see later is in fact the minimum of H + \nabla H (x-x_0) + (x-x_0)^\top B (x-x_0)
            \begin{align}\label{eq:convergence_final_result}
                \Hhat(\vx) - \Hhat(\vy) \le & \nabla \Hhat(\vy)^\top (\vx - \vy) + 2\|\hat{\mQ}^{\frac{1}{2}} (\vx - \vy) \| \| \hat{\mQ}^{\frac{1}{2}} (\vx - \vy) \| \\
                = & (2\eta^2 - \eta) \nabla \Hhat(\vy)^\top \hat{\mQ}^{-1}\nabla \Hhat(\vy)
            \end{align}
            which is less or equal to $0$ if $\eta \in [0, \frac{1}{2}]$ given $\hat{D}^{-1}$ being positive semi-definite, and thus the convergence of our MM algorithm at $\eta = \frac{1}{2}$. 
            \par
            
    \subsection{Miscellaneous}
        \paragraph{Bounded $\lambda$}
        For hyperparameters to be bounded, we can define $\lambda = \frac{1}{1 + \hat{\lambda}}$ and thus $\hat{\lambda} = \frac{1}{\lambda} - 1$ so that
        \begin{align}
            \mF^{(k+1)} =& (\text{diag}(\vq) + \hat{\lambda}\mI)^{-1} ( \mW\odot\tilde{\mA}) \mF^{(k)} +  (\text{diag}(\frac{\vq}{\hat{\lambda}}) + \mI)^{-1} \mF^{(0)} \\
            =& (\text{diag}(\vq) +(\frac{1}{\lambda} - 1)\mI)^{-1} ( \mW\odot\tilde{\mA}) \mF^{(k)} +  (\text{diag}(\frac{\lambda\vq}{1 - \lambda}) + \mI)^{-1} \mF^{(0)}.
        \end{align}
    
        % \paragraph{Wrong Implementation}
        % Besides the normalization of features used in the calculation of $\mW$, previous results from my code (mimicking code from \citet{yang_graph_2021}) treat $\text{diag}(\vq)$ as if it were $\mI$ but added an additional normalization of $mW\odot\mA$ afterward.
    
        \paragraph{Weiszfeld Reweighting}
        When $\hat{\lambda} = 0$ and $\rho(z) = z$, $\mW_{ij} = 1 / 2z_{ij}$ ($l_{21}$ norm), each element $\vq_i = \sum_{j} \frac{1}{2z_{ij}d_i}$ in the preconditioner $\hat{\mQ}^{-1}$ shares some similarity with the weighting factor in the Weiszfeld method which is intended to find the geometric median.
